# Supplementary material for: Dynamic Graph Representation Learning with Neural Networks: A Survey
Source: arXiv:2304.05729 source file (2023-04-12)
Supplement: Supplementary file 2 [file 99-Appendix-NN.tex]

\section{Static Graph Encoding}
\label{sec:FundaNN-GNN}
For a long time, static graph representation learning have been based on matrix factorisation \cite{yang2008non,sarkar2011community,ahmed2013distributed,cao2015grarep,ou2016asymmetric} and random walks \cite{page1999pagerank,jeh2002simrank,mikolov2013efficient,perozzi2014deepwalk,tang2015line,grover2016node2vec}. Recently, graph neural networks have emerged as powerful approaches, thanks to their ability to learn adaptive parameters to map and filter the signals on the graph. In the following, we split the graph representation learning methods into Random Walk-based, Matrix Factorisation-based, and GNN-based.

% \begin{figure}[!ht]
% 	\centering
% 	\includegraphics[width=\columnwidth]{figs/3_g_enc_traditional.jpg}
% 	\caption{Traditional methods for static graph encoding. Left: Illustration of random walk method. The sequences of nodes are sampled and passed into a "Word2Vec" like approach to obtain the hidden state of each node. Right: Illustration of matrix factorization. A sparse user-item matrix of $n \times m$ size is decomposed to obtain the user representations ($n \times k$) and the item representations ($k \times m$).}
%  	\label{FIG:genc_trad}
% \end{figure}

\subsection{Random Walk-based}
After first introduced by Karl in 1905 \cite{pearson1905problem}, Random walk-based approaches have then been applied to graph structure sampling. Its variants have been employed for applications including node similarity computation \cite{tong2006fast}, search engines \cite{page1999pagerank}, and so on for more than two decades.

A simple example is to randomly sample multiple sequences of nodes by starting from several nodes and walking to their neighbouring nodes with probability $1-a$ or jumping randomly to any node in the graph with probability $a$. These sequences of nodes can be transformed into attribute vectors of nodes by various methods, such as Skip-Gram model \cite{tang2015line} or embedding by neural networks \cite{perozzi2014deepwalk,grover2016node2vec}. Similar to \textbf{Word2Vec} \cite{mikolov2013efficient} which generates word embeddings based on word co-occurrence frequencies in natural language processing tasks, \textbf{DeepWalk} \cite{perozzi2014deepwalk} and \textbf{Node2Vec} \cite{grover2016node2vec} encode the node embedding according to the sampled node sequences.

\subsection{Matrix Factorisation-based}
Influenced by the idea of dimensionality reduction, there is a category of Matrix Factorisation-based models \cite{ahmed2013distributed}\cite{cao2015grarep}\cite{ou2016asymmetric} in the early research of graph machine learning. For example, \textbf{Graph Factorization} \cite{ahmed2013distributed} encodes the features $\textbf{x}_i, \textbf{x}_j$ of nodes $i, j$ as vectors $\textbf{z}_i, \textbf{z}_j$ and minimises the difference between their inner product $\bigl< \textbf{z}_i,\textbf{z}_j \bigr>$ and their edge weight $a_{ij}$. Matrix factorisation as a kind of shallow embedding method has many limitations: The learned parameters are the embedding of the nodes thus this method is transductive, in addition, matrix factorisation is computationally expansive \cite{chami2020machine}. %Nevertheless, their ideas have inspired a number of later research.

\subsection{GNN-Based}
Geometric deep learning \cite{bronstein2017geometric}, also known as graph neural networks, have recently emerged as an alternative to traditional methods. Benefiting from the rapid development of the technical and scientific environment: efficient learning algorithms, optimized libraries allowing parallel computing on GPUs and dedicated hardwares, they can iterate over the given inputs and outputs to learn the parameters which encode the input features into low-dimensional informative vectors.

Convolutional neural networks (CNNs) \cite{lecun1995convolutional} are one of the most popular neural networks because of their capability to weightedly aggregate the neighbourhood's features and filter signals. One primary problem with graph neural networks is how to define the convolution on a graph. Different perspectives have led to different implementations %(fig. \ref{FIG:genc_gnn})
: (1) spectral convolution and (2) spatial convolution (or message passing), as well as more complex frameworks like (3) graph Autoencoders and (4) graph Transformers.

% \begin{figure}[!ht]
% 	\centering
% 	\includegraphics[width=\columnwidth]{figs/3_g_enc_gnn.jpg}
% 	\caption{Typical GNNs: 1. Spectral convolution performs a Fourier transform on the graph, then multiplies its spectrum with the learnable parameters and then returns it to the node domain. The whole process can be understood as signal filtering on the graph. 2. For a target node $i$, spatial convolution aggregates the attributes of the neighboring nodes to update the its hidden states. 3. Graph (variational) Autoencoder encodes attributes \textbf{X} into hidden states \textbf{Z} and tends to reconstruct $\hat{\textbf{X}}$ or the adjacency matrix $\hat{\textbf{A}}$. 4. Self-attention mechanism (or graph Transformer) adaptively computes weights when aggregating neighbor information according to their hidden states of neighbor nodes.}
%  	\label{FIG:genc_gnn}
% \end{figure}

From a signal processing point of view, the eigenvectors of the normalized Laplacian matrix of a graph can be considered as the bases of its graph Fourier transform. Multiplying the signal of a transformed node (i.e., a spectrum) in the spectral domain by a signal with learnable parameters (i.e., a convolution kernel) is equivalent to a spectral convolution on the graph. Examples are \textbf{Spectral CNN} \cite{bruna2013spectral} and its low-order approximation \textbf{ChebNet} \cite{defferrard2016convolutional}, \textbf{GCN} \cite{kipf2016semi}.

Otherwise, from the spatial point of view, the convolution on the graph can be regarded as the convolution of the image, but is more complicated due to the irregular grid. Thus spatial convolution can be implemented by message passing between connected nodes e.g. \textbf{MPNN} \cite{gilmer2017neural}, \textbf{NN4G} \cite{micheli2009neural}, \textbf{GraphSage} \cite{hamilton2017inductive}, etc. \textbf{GAT} \cite{velivckovic2017graph} adds the attention mechanism to spatial convolution so that a node aggregates information with different weights according to the attributes of neighboring nodes.
Some other approaches incorporate recurrent neural networks and gating mechanisms, such as Gated graph neural network (\textbf{GGNN}) \cite{li2015gated}, combining Gated Recursive Unit (\textbf{GRU})\cite{chung2014empirical} and message passing network, treats message propagation as the recursive update of the hidden states of nodes and controls the update through a gating mechanism.

To encode data \textbf{X} to a latent representation \textbf{Z}, Autoencoder methods tend to reconstruct $\hat{\textbf{X}}$ with encoded \textbf{Z}. When getting $\hat{\textbf{X}}$ and \textbf{X} as similar as possible, Autoencoder learns the parameters which encode the most informative representation \textbf{Z}. A typical example on graphs, Variational Graph Auto-Encoders (\textbf{VGAE}) \cite{kipf2016variational} encodes the feature matrix \textbf{X} and the adjacency matrix $\textbf{A} \in \mathbb{R}^{|V| \times |V|}$ into $\textbf{Z} \in \mathbb{R}^{|V| \times d_V}$ with a two-layer GCN, and then reconstructs the adjacency matrix $\hat{\textbf{A}}$ by an inner-product of \textbf{Z}, i.e., $\sigma(\textbf{Z}.\textbf{Z}^\mathrm{T})$.

In addition to the above models, Transformer models have been applied to graphs in recent years. Min et als. \cite{min2022transformer} summarizes them as the combinations of the following three approaches: (1) Transformer as auxiliary modules of GNN \cite{ying2021transformers,rong2020self,zhang2020graph}, (2) Use of graph topology for improving self-attention \cite{ying2021transformers,zhang2020graph}, such as using the adjacency matrix as a mask, (3) Use of graph structure during the positional encoding \cite{zhao2021gophormer,tholke2022torchmd}, such as degree or spectrum of nodes.

Once the graph is encoded into a latent representation \textbf{Z}, classical tasks such as classification or regression can be performed by a "readout" operation that aggregates information. This can be performed using different pooling methods \cite{ying2018hierarchical} \cite{gao2021topology}. A very common case is to use mean pooling to take the average value of the attributes of all nodes as the attributes of the entire graph \cite{bronstein2017geometric}.

% In the case of heterogeneous graphs, it is common to map different types of nodes to the same dimensional vector space to facilitate operations.

Despite the great performance of these model components on various static graph tasks, there are more additional elements to consider when handling dynamic graphs, which are the encoding of temporal and sequential data.

\section{Sequential And Temporal Data Encoding With NNs}
\label{sec:FundaNN-RNN}
The time information on a dynamic graph may be indexes of the sequence (in STGs and DTDGs) or precise timestamps (in CTDGs), or both. 
In the literature, neural networks encode sequential or temporal data in different ways, we present the more classical ones in the following. %(as shown in fig. \ref{FIG:t_enc}).

\subsection{Encoding Sequential Data}
There is a semantic dependency between the elements of sequential data, as in natural language processing tasks. 
To handle them, the most well-known one is Recurrent Neural Network (\textbf{RNN}) \cite{hopfield1982neural} which processes each input element recursively along the direction of the sequence. By adding the gating mechanism, Long Short-Term Memory (\textbf{LSTM}) \cite{hochreiter1997long} \cite{gers2001long} and Gated Recursive Unit (\textbf{GRU})\cite{chung2014empirical} have better performance on long sequences.

Recursive networks like RNNs are not suitable for parallel computing, while parallelizable networks based on linear operations and convolution can avoid or reduce the number of sequential operations: Equally using gating mechanism, the Gated Linear Units (\textbf{GLU}) \cite{dauphin2017language} computes the hidden states of the gated input by convolution to avoid dependence on the previous time steps. Some other models use purely convolutional layers, such as causal convolution in \textbf{WaveNet} \cite{oord2016wavenet}, which encodes the signal of the last $l$ time steps through $l$ layers of convolution. When processing long sequences, dilated causal convolution \cite{yu2015multi,zhang2019multi} expands the field of perception to avoid too many layers.

Furthermore, \textbf{self-attention} \cite{vaswani2017attention} modules, better known with the Transformer architecture, can also capture long-term dependencies by using linear transforms to learn the influence of each element in a sequence on each other.

\subsection{Encoding Time Information}
Since time $t$ is a numerical value, another practical way is to encode the timestamp or sequence number as a $d$-dimensional vector as part of the input features.

Common approaches are \textbf{Positional Encoding} (PE) \cite{vaswani2017attention} which is employed in Transformer architecture, and \textbf{Time2Vec} \cite{kazemi2019time2vec} which especially focused on encoding temporal patterns \cite{skarding2021foundations}. Both of them use sine or cosine functions, which make the vector representation bounded and smoothly continuous in each dimension, as well as guarantee the translational invariance of time difference values.  
Another class of methods, Temporal Point Process (\textbf{TPP} \cite{lewis1972multivariate}), models the intensity function $\lambda_i(t)$ of the probability of event $i$ occurring at moment $t$ based on the historical events. Neural networks allow TPP to learn intensity functions automatically to better fit actual situations.

% \break
